# Supplementary material for: Emergence of Communication in an Interactive World with Consistent Speakers
Source: arXiv:1809.00549 source file (2019-03-24)
Supplement: Supplementary file 1 [file appendix_pass.tex]

\appendix
\section{Implementation Details}
We train the agents simultaneously in 10 different environments for up to a total of 10 million steps. Parameters are updated in a batch every 5 steps using RMSProp \cite{Tieleman2012}, with a learning rate of 4e-4 for the speaker and 1e-3 for the listener. We use a hidden state size and GRU cell size of 50.

\subsection{Network architecture}

The listener receives as input the world-utterance pair $(w_t, \bu)$, with the world $w_t$ given as raw RBG pixel values (15x15x3 values from 0 to 1) and then goes through {\em the same} convolutional layer $Conv_1$. We used 6 filters, a kernel size of 3 and strides of 3 in all setups.
\begin{align*}
\hat{w}_t &= Conv_1(w_t) \\
\hat{i}_t &= Conv_1(i_t)
\end{align*}
Each symbol $u_i \in \bR^{|\sV|}$ of the utterance $u$ is represented as a one-hot vector. We embed each symbol using an embedding matrix $W \in \bR^{|\sV|\times d}$:
$$ \hat{u_i} = u_i \cdot W$$
We can then use either one of the two following models to get a representation for the entire utterance:
%either use a BOW model by summing the embedded symbols: 
\begin{align}
\hat{r}_u &= \frac{1}{|u|} \cdot \sum_i{\hat{u_i}} \\
\hat{r}_u &= \text{GRU}(\hat{u_i})
\end{align}
Where (1) is a bag-of-words averaging model and (2) is a GRU model \cite{cho2014properties} with the last hidden state taken as output. The final representation vector for $\bu$ is calculated using a feed-forward layer:
$$r_u = FF_1(\hat{r}_u)$$
We then use multiplicative interaction between the world and utterance (in a similar way to \citet{oh2015action}). The intuition behind it is that we want the way the agent observes the world to be dependent on the goal. While it is possible to do so with a feed forward layer on the concatenated world and utterance representations, the multiplicative way allows to do so without the price of additional parameters. The world representation $\hat{w}_t$ is  transposed and reshaped to be in the form $n_w \in \bR^{c, l}$, where $l$ is the number of used filters in $Conv_1$ - in this case 6 - and $c$ is the total output cells of the convolution result. We do the same for the inventory representation $n_i$. The utterance representation $\hat{r}_u$ is reshaped to be in the form $n_u \in \bR^{l, k}$, where $l$ is again the number of filters and $k$ is dependent on $d$ (note that we impose a spatial structure on $r_u$). We normalize (l2) $n_w$ and $n_u$ and multiply the matrices:
\begin{align*}
m_w &= n_w \cdot n_u \\
m_i &= n_i \cdot n_u
\end{align*}
The output $m_w$ then goes through another convolutional layer $Conv_2$ (by reformatting the vector to the appropriate dimensions), with 8 layers, a kernel size of 3 and a stride of 1. It is then concatenated with $m_i$ and goes through a feed forward layer to get a final hidden representation $h$ of the inputs:
$$h = FF_2([Conv_2(m_w), m_i])$$
Finally, the value $v$ and action $a$ are obtained using a linear layer that outputs a scalar and a softmax layer of size $|\sA|$, respectively.

The speaker's model is similar to the listener's model described above, with the following difference: The speaker's input is a world-goal pair $(w_0,g)$, and to calculate $r_g$ we simply use $Conv_1$. The speaker then uses $r_g$ instead of $r_u$ for the rest of the calculations to obtain a hidden representation $h_g$ for the input task.

When training the speaker with policy gradient (marked as dashed red box), the utterance $\bu$ is generated with a GRU, that receives $h_g$ as its initial hidden state. When training with \cco{}, $\bu$ is given as a third input to the network (marked as a dotted purple box), and a representation $h_u$ is computed. The distance $d$ with $h_g$ is then calculated.
