# Supplementary material for: Emergence of Communication in an Interactive World with Consistent Speakers
Source: arXiv:1809.00549 source file (2019-03-24)
Supplement: Supplementary file 2 [file appendix.tex]

\appendix
\section{Implementation Details}
We train the agents simultaneously in 10 different environments for up to a total of 10 million steps. Parameters are updated in a batch every 5 steps using RMSProp \cite{Tieleman2012}, with a learning rate of 4e-4 for the speaker and 1e-3 for the listener. We use a hidden state size and GRU cell size of 50.
